# Supplementary material for: Decoding Decoders: Finding Optimal Representation Spaces for Unsupervised Similarity Tasks
Source: arXiv:1805.03435 source file (2018-05-09)
Supplement: Supplementary file 1 [file optimisation.tex]

\section{Optimising the objective maximises the dot product}
\label{sec:appendix-opt}
The task is to maximise the quantity $Q$ found in  \cref{eq:mle_log_linear}
\begin{equation}
  Q =
  \sum_{(s_i,c_i)\in D} \sum_{w\in c_i} \left[ \mbu_w\cdot\mbh_{i} - \log{\sum_{w^\prime\in V_W}\exp{(\mbu_{w^\prime}\cdot\mbh_{i})}}\right] =
  \sum_{(s_i,c_i)\in D} \sum_{w\in V_W} q_{iw},
\end{equation}
where
\begin{equation}
  \label{eq:optimisation}
  q_{iw} = \log{(x)} - \log{(x+y)},
\end{equation}
where we drop the sentence and word subscript on $x$ and $y$ for brevity (but in
the following equations it is understood we are referring to a specific given
word $w$ given specific sentence $s$), and
\begin{align}
  x & = \exp{(\mbu_w\cdot \mbh_{i})}, &
  y & = \sum_{w^\prime\in |V_W| \setminus \{w\}} \exp{(\mbu_{w^\prime}\cdot \mbh_{i})}.
\end{align}
We find the derivatives
\begin{align}
  \frac{\partial q_{s_iw}}{\partial x} &= \frac{y}{x(x+y)}, &
  \frac{\partial q_{s_iw}}{\partial y} &= - \frac{1}{(x+y)},
\end{align}
and conclude that since both $x$ and $y$ are therefore positive, that for a given word $w$ and sentence $s_i$, the quantity
$q_{s_iw}$ is made larger by
\begin{itemize}
  \item Increasing $x$, leading to an increase in the dot product of the word present in the
    context with the context vector, and
  \item Reducing $y$, leading to a decrease in the dot products of all other
    words.
\end{itemize}
Performing this analysis across all words in a context leads to the maximisation
of the dot products of the context representation $\mbc_i$ with the sentence
representation $\mbh_i$
\begin{equation*}
  \sum_{w\in c_i} \mbu_w\cdot \mbh_{i} = \mbc_{i} \cdot \mbh_{i}
\end{equation*}
and a minimisation of the dot product of the sentence representation $\mbh_i$
word vectors $\mbu_{w^\prime}$ that are not in the context $c_i$
\begin{equation*}
  \sum_{w\in c_i} \log \sum_{w^\prime\in |V_W| \setminus \{w\}} \exp{(\mbu_{w^\prime}\cdot \mbh_{i})}.
\end{equation*}
