# Supplementary material for: Decoding Decoders: Finding Optimal Representation Spaces for Unsupervised Similarity Tasks
Source: arXiv:1805.03435 source file (2018-05-09)
Supplement: Supplementary file 2 [file unrolled.tex]

\section{Unrolled RNN Results}
\label{sec:appendix-unroll}

\input{tables/similarity_unrolled}
